# Supplementary material for: Robust Distributed Arrays: Provably Secure Networking for Data Availability Sampling
Source: arXiv:2504.13757 source file (2025-04-22)
Supplement: Supplementary file 1 [file additional.tex]

\ifnum\submission=1
	\usepackage[pdfpagelabels=true,linktocpage=true,colorlinks=true]{hyperref}
\else
	\usepackage[pdfpagelabels=true,linktocpage=true,pagebackref,colorlinks=true]{hyperref}
	\ifnum\llncs=0
		\renewcommand*{\backref}[1]{(Cited on Page~#1.)}
	\fi
\fi % If submission=1: pagebackrefs are deactivated
	% If submission=0 and not using lncs `Cited on page...' is added to each entry in hte biblio

% ---------------------------------------------------------------------
\def\titleofpdf{\titletext}		%automatically embeds the title into pdf info. Part 1
\def\authorsofpdf{%				%automatically embeds the author names your pdf info. Part 1
\ifcsname 5name\endcsname
	\csname 1name\endcsname~et~al.
\else
	\ifcsname 1name\endcsname
		\csname 1name\endcsname
		\ifcsname 3name\endcsname
			,\ \csname 2name\endcsname
			\ifcsname 4name\endcsname
				,\ \csname 3name\endcsname\ and \csname 4name\endcsname
			\else%
				\ and\ \csname 3name\endcsname
			\fi
		\else
			\ifcsname 2name\endcsname
				\csname 2name\endcsname
			\fi
		\fi
	\fi
\fi
}

\ifnum\submission=1 %link colours are set to black when submission=1
	\hypersetup{
	pdftitle={\titleofpdf}, %embedding of title into pdf info. Part 2
	pdfauthor=\ifnum\anonymous=0{\authorsofpdf}\else{}\fi, %author pdf info embed. when not anonym.
	linkcolor=[rgb]{0,0,0}, %link colours are set to black.
	urlcolor=[rgb]{0,0,0},  %link colours are set to black.
	citecolor=[rgb]{0,0,0}  %link colours are set to black.
	}
\else
	\hypersetup{
	pdftitle={\titleofpdf},
	pdfauthor=\ifnum\anonymous=0{\authorsofpdf}\else{}\fi,
	linkcolor=[rgb]{0,0,0.5},
	urlcolor=[rgb]{0,0,0.5},
	citecolor=[rgb]{0,0,0.5}
	}
\fi
% ---------------------------------------------------------------------

%load cleveref always after hyperref
\ifnum\abbrevref=0
	\usepackage[capitalise,noabbrev]{cleveref}
\else
	\usepackage[capitalise]{cleveref}
\fi

\usepackage{nicodemus}
\usepackage[absolute]{textpos}	% used for warning messages and publication info
\usepackage{everypage}			% used for the page limit warning



\ifnum\LNCSpreview=1 %LNCS review reminder watermark
	\usepackage[paperwidth=152mm,paperheight=235mm,textwidth=122mm,textheight=193mm]{geometry}
	\AddEverypageHook{
		\begin{textblock}{1}[1,1](0.5,0.9)
			\centering\Large
			\textcolor{lightgray}{\textbf{LNCS Preview mode active.}}
		\end{textblock}
	}
	\def\choosepubinfo{0}
\fi

\ifnum\overflow=1
	\overfullrule=2mm
\fi

\ifnum\allowbreaks=1
	\allowdisplaybreaks
\fi

\ifnum\showlabels=1
	\usepackage{showkeys}
\fi

\ifnum\submission=1
	\def\authnotes{0}
\fi

\ifnum\anonymous=1
	\def\authnotes{0}
\fi

\ifx\pagelimit\empty %page limit warning magic
\else
	\newcounter{pagewarning}
	\setcounter{pagewarning}{\pagelimit}
	\AddEverypageHook{
		\ifnum\thepage>\thepagewarning
			\ifnum\LNCSpreview=0
				\begin{textblock}{1}[0.5,0](0,-13.5)
			\else
				\begin{textblock}{1}[0.5,0](0,-11.95)
			\fi
				\centering\Large
				\textcolor{red}{\textbf{This page is exceeding the page limit.}}
			\end{textblock}
		\fi
}
\fi

\def\notesindocument{0}

\newlength{\strutdepth}%
\settodepth{\strutdepth}{\strutbox}%

\newcommand{\notes}[3]{ %framework for margin notes of any kind
\ifnum\authnotes=1
	\def\notesindocument{1}%
	\noindent{%\bfseries
	\color{#1}{#3}\color{#1}}%
	\strut\vadjust{\kern-\strutdepth%
		\vtop to \strutdepth{%
			\baselineskip\strutdepth%
			\vss\llap{{\large\color{#1}\textbf{#2}\quad\color{black}}}\null%
		}%
	}%
\fi
}

% below you see how to set up margin notes. hspace hack for using paper size cropped to lncs size
\ifnum\LNCSpreview=0
	\newcommand{\todo}[1]{\notes{Red}{TODO}{#1}}
	\newcommand{\new}[1]{\notes{ForestGreen}{NEW}{#1}}
	\newcommand{\alert}[1]{\notes{Red}{ALERT}{#1}}
	\newcommand{\authornote}[1]{\notes{black}{NOTE}{#1}}
\else
	\newcommand{\todo}[1]{\notes{Red}{Todo\hspace{-1.5ex}}{#1}}
	\newcommand{\new}[1]{\notes{ForestGreen}{New\hspace{-1.5ex}}{#1}}
	\newcommand{\alert}[1]{\notes{Red}{Alert\hspace{-1.5ex}}{#1}}
	\newcommand{\authornote}[1]{\notes{black}{Note\hspace{-1.5ex}}{#1}}
\fi

\newcommand{\authnote}[2]{ %command for authnotes that appear in the text body
	\ifnum\authnotes=1
		\def\notesindocument{1}
		\begin{center}
			\fbox{%
				\begin{minipage}{.98\textwidth}
					\textbf{#1 says:} #2\authornote{}
				\end{minipage}%
			}
		\end{center}
	\fi
}

\ifnum\llncs=1
	\ifnum\llncsqedsymbol=1
		\let\oldproof\proof
		\renewenvironment{proof}%
		{\begin{oldproof}}%
		{\qed\end{oldproof}}
	\fi
\fi

%
\ifnum\llncs=0				%definition of new environemnt styles when not using llncs
\usepackage{newpxtext} %\usepackage[euler-digits]{eulervm}

\newtheoremstyle{mytheorem}
  {\topsep} % Space above
  {\topsep} % Space below
  {} % Body font
  {} % Indent amount
  {\bfseries} % Theorem head font
  {} % Punctuation after theorem head
  {.5em} % Space after theorem head
  {\thmname{#1}\thmnumber{ #2}\thmnote{ {\bfseries (#3)}}.} % Theorem head spec

\newtheoremstyle{myplain}
  {\topsep} % Space above
  {\topsep} % Space below
  {\itshape} % Body font
  {} % Indent amount
  {\bfseries} % Theorem head font
  {} % Punctuation after theorem head
  {.5em} % Space after theorem head
  {\thmname{#1}\thmnumber{ #2}\thmnote{ {\normalfont(#3)}}.} % Theorem head spec

\newtheoremstyle{mydefinition}
  {\topsep} % Space above
  {\topsep} % Space below
  {} % Body font
  {} % Indent amount
  {\bfseries} % Theorem head font
  {} % Punctuation after theorem head
  {.5em} % Space after theorem head
  {\thmname{#1}\thmnumber{ #2}\thmnote{ {\normalfont(#3)}}.} % Theorem head spec

\newtheoremstyle{myremark}
  {} % Space above
  {} % Space below
  {} % Body font
  {} % Indent amount
  {\itshape} % Theorem head font
  {} % Punctuation after theorem head
  {.5em} % Space after theorem head
  {\thmname{#1}\thmnumber{ #2}\thmnote{ {\normalfont(#3)}}.} % Theorem head spec

	\theoremstyle{mytheorem}				% new theorem-like environments when llncs=0
	\newtheorem{theorem}{Theorem}

	\theoremstyle{myplain}
	\newtheorem{lemma}{Lemma}
	\newtheorem{corollary}{Corollary}
	\newtheorem{proposition}{Proposition}
	\newtheorem{construction}{Construction}
	\newtheorem{conjecture}{Conjecture}

	\theoremstyle{mydefinition}
	\newtheorem{definition}{Definition}
	\newtheorem{claim}{Claim}
	\newtheorem{assumption}{Assumption}
	\newtheorem{fact}{Fact}

	\theoremstyle{myremark}
	\newtheorem{remark}{Remark}
	\newtheorem{example}{Example}
	\newtheorem{note}{Note}
	\newtheorem{observation}{Observation}
\else									% new theorem-like environments when llncs=1
	\spnewtheorem{construction}[theorem]{Construction}{\bfseries}{}
	\spnewtheorem{assumption}[theorem]{}{\bfseries}{}
	\spnewtheorem{fact}[theorem]{Fact}{\bfseries}{}

	\spnewtheorem{observation}[theorem]{Observation}{\itshape}{}
\fi

% to save some typing
\newenvironment{theo}{\begin{theorem}}{\end{theorem}}
\newenvironment{thm}{\begin{theorem}}{\end{theorem}}
\newenvironment{lemm}{\begin{lemma}}{\end{lemma}}
\newenvironment{lem}{\begin{lemma}}{\end{lemma}}
\newenvironment{coro}{\begin{corollary}}{\end{corollary}}
\newenvironment{cor}{\begin{corollary}}{\end{corollary}}
\newenvironment{prop}{\begin{proposition}}{\end{proposition}}
\newenvironment{conj}{\begin{conjecture}}{\end{conjecture}}
\newenvironment{clai}{\begin{claim}}{\end{claim}}
\newenvironment{defi}{\begin{definition}}{\end{definition}}
\newenvironment{defn}{\begin{definition}}{\end{definition}}
\newenvironment{assu}{\begin{assumption}}{\end{assumption}}
\newenvironment{rema}{\begin{remark}}{\end{remark}}
\newenvironment{rem}{\begin{remark}}{\end{remark}}
\newenvironment{cons}{\begin{construction}}{\end{construction}}
\newenvironment{obse}{\begin{observation}}{\end{observation}}
\newenvironment{fct}{\begin{fact}}{\end{fact}}


\ifnum\abbrevref=0			%Tell cleveref what words to use in front of a reference (abbrevref=0)
	\crefname{assumption}{Assumption}{Assumptions}
	\crefname{construction}{Construction}{Constructions}
	\crefname{corollary}{Corollary}{Corollaries}
	\crefname{conjecture}{Conjecture}{Conjectures}
	\crefname{definition}{Definition}{Definitions}
	\crefname{exmaple}{Example}{Examples}
	\crefname{lemma}{Lemma}{Lemmata}
	\crefname{observation}{Observation}{Observations}
	\crefname{proposition}{Proposition}{Propositions}
	\crefname{remark}{Remark}{Remarks}
	\crefname{theorem}{Theorem}{Theorems}
\else						%Tell cleveref what words to use in front of a reference (abbrevref=1)
	\crefname{assumption}{Ass.}{Ass.}
	\crefname{construction}{Constr.}{Constr.}
	\crefname{corollary}{Cor.}{Cor.}
	\crefname{conjecture}{Conj.}{Conj.}
	\crefname{definition}{Def.}{Def.}
	\crefname{exmaple}{Ex.}{Ex.}
	\crefname{lemma}{Lem.}{Lem.}
	\crefname{observation}{Obs.}{Obs.}
	\crefname{proposition}{Prop.}{Prop.}
	\crefname{remark}{Rem.}{Rem.}
	\crefname{theorem}{Thm.}{Thms.}
\fi

\crefname{claim}{Claim}{Claims}
\crefname{fact}{Fact}{Facts}
\crefname{note}{Note}{Notes}

%Super Mario coin version of \getsr
\def\YYYSMcoin{\mbox{\begin{tikzpicture}[scale=0.0125]
\definecolor{coinbrown}{HTML}{D89E36}\definecolor{coindarkyellow}{HTML}{F8D81E}\definecolor{coinyellow}{HTML}{F8F800}\fill[coinyellow] (3,-1) rectangle (9,9);\fill(0,0) rectangle (1,8);\fill(1,8) rectangle (2,10);\fill(2,10) rectangle (4,11);\fill(4,11) rectangle (8,12);\fill(8,11) rectangle (10,10);\fill(10,10) rectangle (11,8);\fill(11,8) rectangle (12,0);\fill(10,-2) rectangle (11,0);\fill(8,-3) rectangle (10,-2);\fill(4,-4) rectangle (8,-3);\fill(2,-3) rectangle (4,-2);\fill(1,0) rectangle (2,-2);\fill (5,-1) rectangle (7,0);\fill (7,0) rectangle (8,8);\fill[coinbrown] (9,8) rectangle (10,10);\fill[coinbrown] (10,0) rectangle (11,8);\fill[coinbrown] (9,-2) rectangle (10,0);\fill[coinbrown] (8,-2) rectangle (9,-1);\fill[coinbrown] (4,-3) rectangle (8,-2);\fill[coindarkyellow] (2,-2) rectangle (3,8);\fill[coindarkyellow] (3,-2) rectangle (8,-1);\fill[coindarkyellow] (8,-1) rectangle (9,0);\fill[coindarkyellow] (9,0) rectangle (10,8);\fill[coindarkyellow] (8,8) rectangle (9,10);\fill[coindarkyellow] (4,9) rectangle (8,10);\fill[coindarkyellow] (3,8) rectangle (4,9);\fill[coindarkyellow] (5,0) rectangle (7,2);\fill[coindarkyellow] (6,2) rectangle (7,8);\fill[white] (4,0) rectangle (5,8);\fill[white] (5,8) rectangle (7,9);
\end{tikzpicture}}}

%Die version of getsr
\def\YYYdie{\mbox{\begin{tikzpicture}[scale=0.85,x=1em,y=1em,radius=0.09]
\draw[rounded corners=1,line width=.25pt] (0,0) rectangle (1,1);\fill (0.275,0.275) circle;\fill (0.725,0.725) circle;\fill (0.5,0.5) circle;\fill (0.275,0.725) circle;\fill (0.725,0.275) circle;
\end{tikzpicture}}}

\newcommand{\getsr}{
	\ifnum\dieordollar=0
		\mathrel{\vbox{\offinterlineskip\ialign{
			\hfil##\hfil\cr
			\hspace{0.1em}$\scriptscriptstyle\$$\cr
			$\leftarrow$\cr
		}}}
	\fi
	\ifnum\dieordollar=1
		\mathrel{\vbox{\offinterlineskip\ialign{
			\hfil##\hfil\cr
			{\scalebox{0.5}{\hspace{0.4em}\YYYdie}}\cr
			\noalign{\kern0.05ex}
			$\leftarrow$\cr
		}}}
	\fi
	\ifnum\dieordollar=2
		\mathrel{\vbox{\offinterlineskip\ialign{
			\hfil##\hfil\cr
			\hspace{0.1em}$\YYYSMcoin$\cr
			$\leftarrow$\cr
		}}}
	\fi
}

\newcommand{\testequal}{
	\mathrel{\vbox{\offinterlineskip\ialign{
			\hfil##\hfil\cr
			\hspace{0.1em}$\scriptscriptstyle?$\cr
			$\leftarrow$\cr
		}}}
}
\newcommand{\checkfornotes}{
	\ifnum\notesindocument=1
		\ifnum\LNCSpreview=1
			\begin{textblock}{1}[0.5,0](0,0.25)
		\else
			\begin{textblock}{1}[0.5,0](0,0.85)
		\fi
		\centering
		\textcolor{red}{\large \textbf{There are still unresolved comments in this document.}}
		\end{textblock}
	\fi
}





%%%%%%%%%%%%%%%%%%%%%%%%%%%%%%%%%%%%%%%%%%%%%%%%%%%%%%%%%%%%%%%%%%%%%%%%%%%%%%%%%%%%%%%%%%%
%
%     SOME COMMANDS FOR FONTS
%
%%%%%%%%%%%%%%%%%%%%%%%%%%%%%%%%%%%%%%%%%%%%%%%%%%%%%%%%%%%%%%%%%%%%%%%%%%%%%%%%%%%%%%%%%%%

\newcommand{\varfont}[1]{\mathit{#1}}
\newcommand{\algfont}[1]{\mathsf{#1}}
\newcommand{\termfont}[1]{\mathsf{#1}}
\newcommand{\orfont}[1]{{\ensuremath{\textsc{#1}}}\xspace}
\newcommand{\eventfont}[1]{\mathsf{#1}}
\newcommand{\mat}[1]{\vec{#1}}
